# Supplementary material for: Semantic Image Synthesis with Unconditional Generator
Source: arXiv:2402.14395 source file (2024-02-22)

**Target**

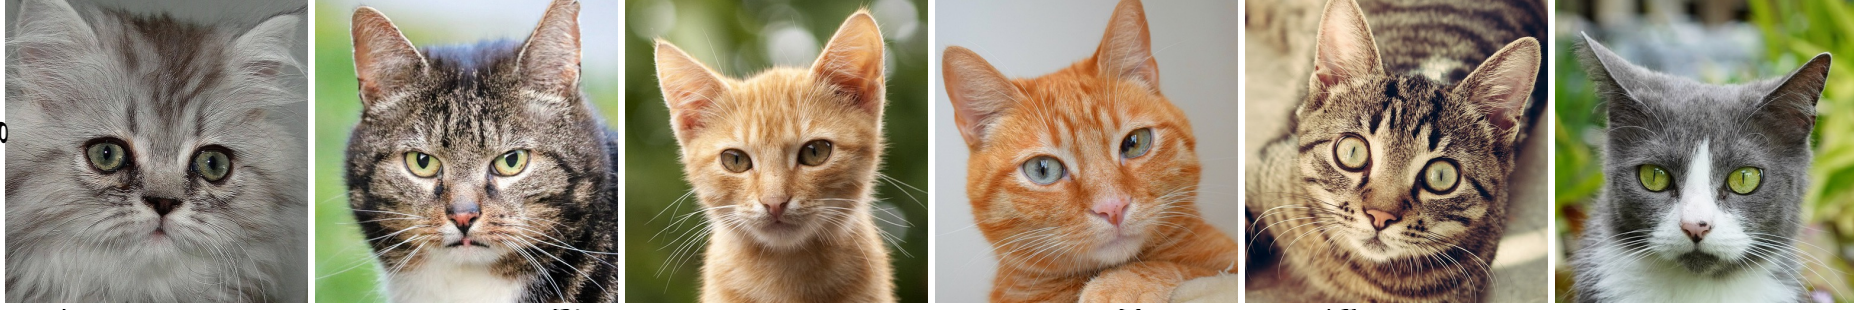

**Sketch**

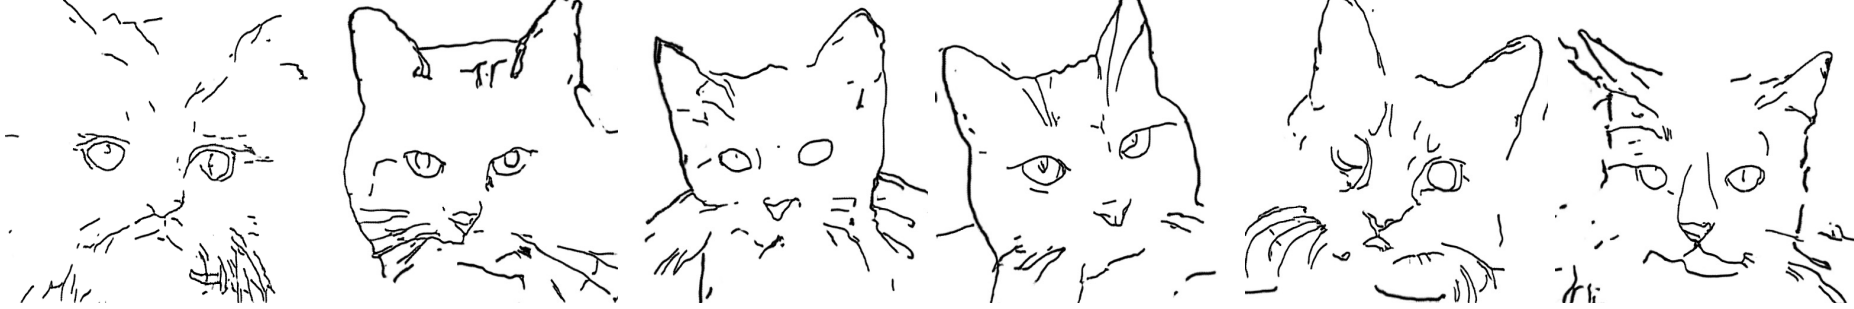

**Style**

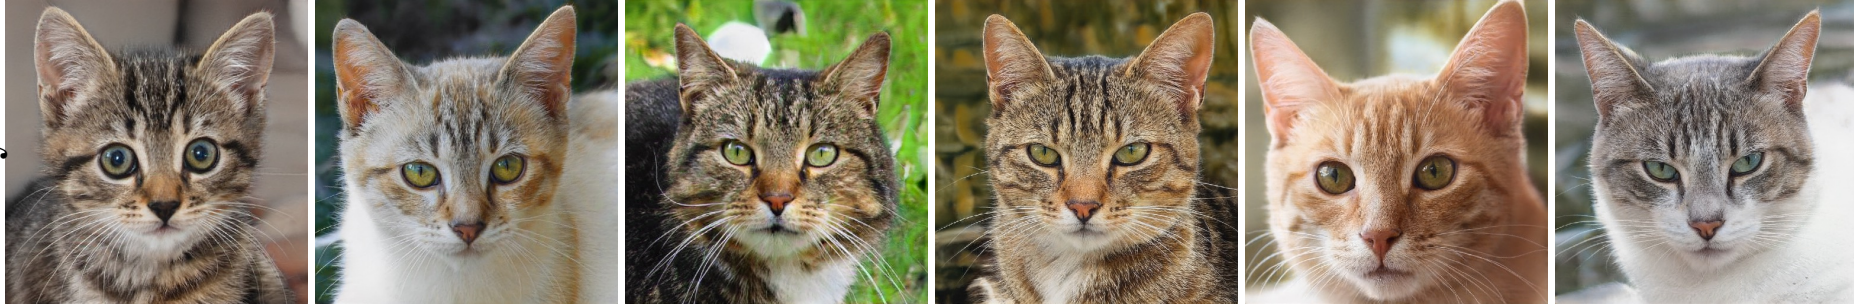

**Ours**

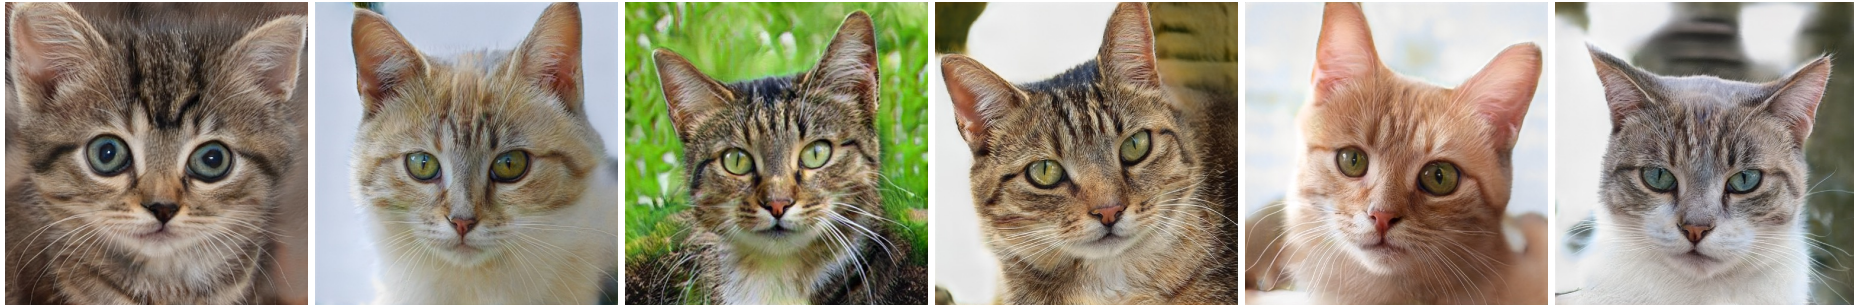



Target

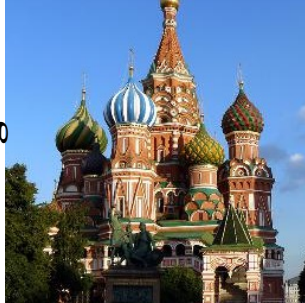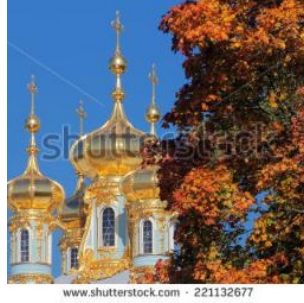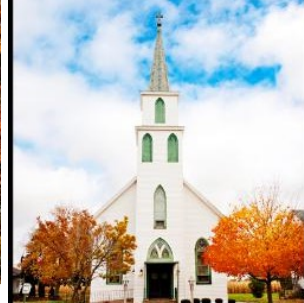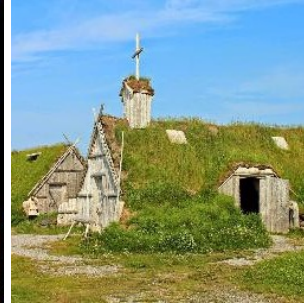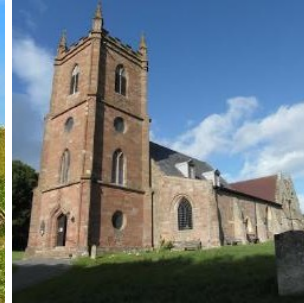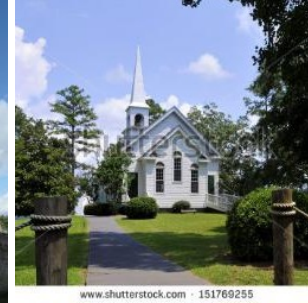

Sketch

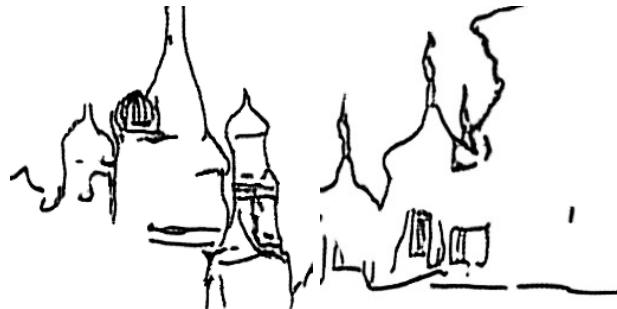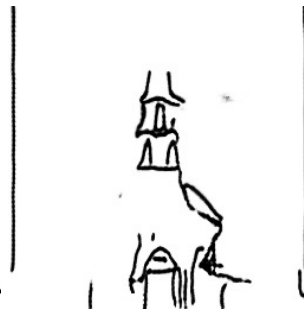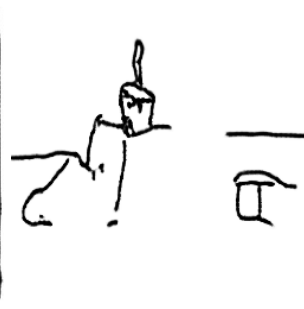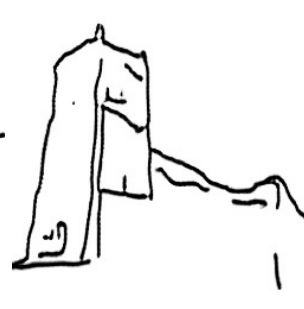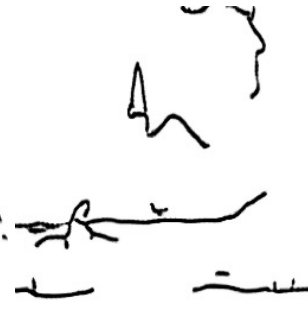

Style

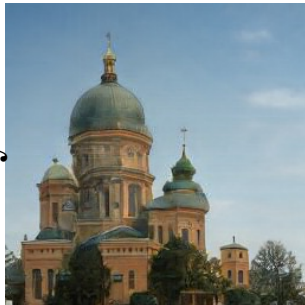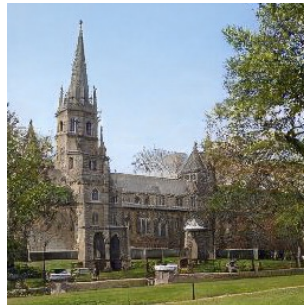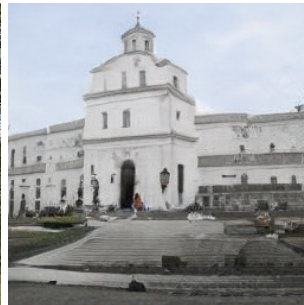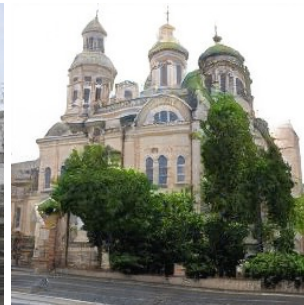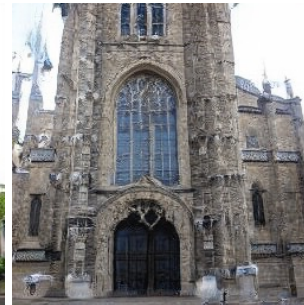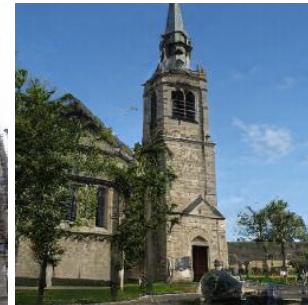

Ours

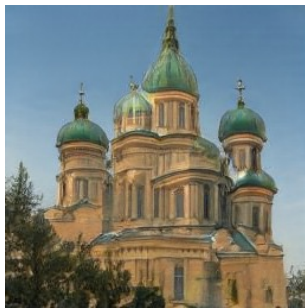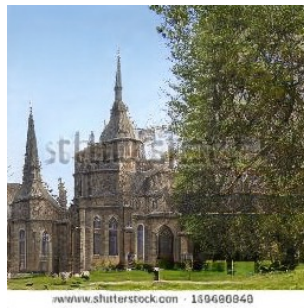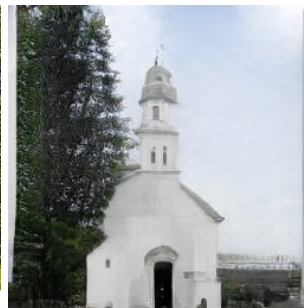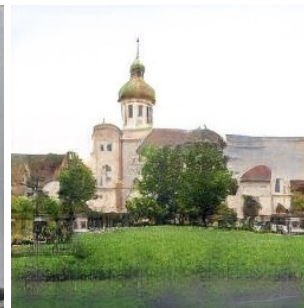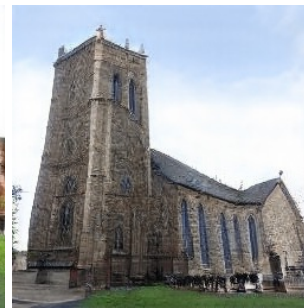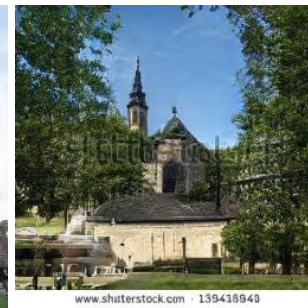

Supplement: Supplementary file 2 [file C_sketch2.pdf]
